# Supplementary material for: Molecular Algebraic Geometry: Electronic Structure of H$_3^+$ as Algebraic Variety
Source: arXiv:2307.02145 source file (2024-05-14)
Supplement: Supplementary file 1 [file supplemental.tex]

\newpage
\section*{Supplementary Materials}

In this part, we show the small program to do the algebraic computation
and the obtained result. 

\subsection*{Script}
\begin{Verbatim}[breaklines=true,breakanywhere=true]
option(noredefine);
LIB "solve.lib";
option(redSB);

//The definition of the ring.
ring r=0,(x, y, z, e),dp;

print("ENERGY FUNCTIONAL OBJ:");
poly OBJ=-20000*e*x**2 - 22288*e*x*y - 22288*e*x*z- 20000*e*y**2 - 22288*e*y*z - 20000*e*z**2 + 20000*e + 7746*x**4 + 14316*x**3*y + 14316*x**3*z + 18392*x**2*y**2 + 26758*x**2*y*z + 18392*x**2*z**2 - 31781*x**2 + 14316*x*y**3 + 26758*x*y**2*z + 26758*x*y*z**2 - 44637*x*y + 14316*x*z**3- 44637*x*z + 7746*y**4 + 14316*y**3*z + 18392*y**2*z**2 - 31781*y**2 + 14316*y*z**3 - 44637*y*z + 7746*z**4 - 31781*z**2 + 17639;
OBJ;

//The list of the derivatives of OBJ by x, y, z, and e. It generates the ideal I
ideal I=0;
for(int i=1;i<=nvars(r);i=i+1){
I=I+diff(OBJ,var(i));
}
print("THE IDEAL THAT GIVES THE QUANTUM STATES IN THE DEGREE REVESE LEXICOGRAPHIC MONOMIAL ORDERING:");
I;
//The standard basis (Groebner basis) of I.
ideal SI=std(I);
print("THE GROEBNER BASIS (IN THE DEGREE REVESE LEXICOGRAPHIC MONOMIAL ORDERING:");
SI;
ring s=0,(x, y, z, e),lp;

// The change of the base ring, with the change of monomial orderings.
setring s;
ideal j=fglm(r,SI);
print("THE GROEBNER BASIS (IN THE LEXICOGRAPHIC MONOMIAL ORDERING) GENERATED BY FGLM ALGORITHM:");
j;
def R=triang_solve(j,50);

setring R;
print("THE NUMERICAL SOLUTIONS THROUGH TRIANGULATION:");
rlist;

setring s;
LIB "triang.lib";
print("THE PRIMARY IDEAL DECOMPOSITION THROUGH TRIANGULATION (IN THE LEXICOGRAPHIC MONOMIAL ORDERING):");
triangM(j);
\end{Verbatim}

\subsection*{Result}
\begin{Verbatim}[breaklines=true,breakanywhere=true]
                     SINGULAR                                 /  Development
 A Computer Algebra System for Polynomial Computations       /   version 4.1.1
                                                           0<
 by: W. Decker, G.-M. Greuel, G. Pfister, H. Schoenemann     \   Feb 2018
FB Mathematik der Universitaet, D-67653 Kaiserslautern        \  Debian 1:4.1.1-p2+ds-4build2
// ** loaded /usr/bin/../share/singular/LIB/solve.lib (4.1.1.0,Dec_2017)
// ** loaded /usr/bin/../share/singular/LIB/ring.lib (4.1.1.0,Dec_2017)
// ** loaded /usr/bin/../share/singular/LIB/primdec.lib (4.1.1.0,Dec_2017)
// ** loaded /usr/bin/../share/singular/LIB/absfact.lib (4.1.1.0,Dec_2017)
// ** loaded /usr/bin/../share/singular/LIB/matrix.lib (4.1.1.0,Dec_2017)
// ** loaded /usr/bin/../share/singular/LIB/nctools.lib (4.1.1.0,Dec_2017)
// ** loaded /usr/bin/../share/singular/LIB/random.lib (4.1.1.0,Dec_2017)
// ** loaded /usr/bin/../share/singular/LIB/poly.lib (4.1.1.0,Dec_2017)
// ** loaded /usr/bin/../share/singular/LIB/elim.lib (4.1.1.0,Dec_2017)
// ** loaded /usr/bin/../share/singular/LIB/general.lib (4.1.1.0,Dec_2017)
// ** loaded /usr/bin/../share/singular/LIB/inout.lib (4.1.1.0,Dec_2017)
// ** loaded /usr/bin/../share/singular/LIB/triang.lib (4.1.1.0,Dec_2017)
ENERGY FUNCTIONAL OBJ:
7746x4+14316x3y+18392x2y2+14316xy3+7746y4+14316x3z+26758x2yz+26758xy2z+14316y3z+18392x2z2+26758xyz2+18392y2z2+14316xz3+14316yz3+7746z4-20000x2e-22288xye-20000y2e-22288xze-22288yze-20000z2e-31781x2-44637xy-31781y2-44637xz-44637yz-31781z2+20000e+17639

THE IDEAL THAT GIVES THE QUANTUM STATES IN THE DEGREE REVESE LEXICOGRAPHIC MONOMIAL ORDERING:
I[1]=30984x3+42948x2y+36784xy2+14316y3+42948x2z+53516xyz+26758y2z+36784xz2+26758yz2+14316z3-40000xe-22288ye-22288ze-63562x-44637y-44637z
I[2]=14316x3+36784x2y+42948xy2+30984y3+26758x2z+53516xyz+42948y2z+26758xz2+36784yz2+14316z3-22288xe-40000ye-22288ze-44637x-63562y-44637z
I[3]=14316x3+26758x2y+26758xy2+14316y3+36784x2z+53516xyz+36784y2z+42948xz2+42948yz2+30984z3-22288xe-22288ye-40000ze-44637x-44637y-63562z
I[4]=-20000x2-22288xy-20000y2-22288xz-22288yz-20000z2+20000

THE GROEBNER BASIS (IN THE DEGREE REVESE LEXICOGRAPHIC MONOMIAL ORDERING:
SI[1]=1250x2+1393xy+1250y2+1393xz+1393yz+1250z2-1250
SI[2]=95133162140791118915022477384291130437198273923568xye+95133162140791118915022477384291130437198273923568xze+95133162140791118915022477384291130437198273923568yze-445385151795113297801964243667094822393170429440000e3+69786547336661619438621362518675205611839541171135xy+69786547336661619438621362518675205611839541171135xz+69786547336661619438621362518675205611839541171135yz-798518946252107642336567335024167547051564515840000e2-332938241761858584449862911632268468259824966970000e+1933872647058608653746415654726341110916311162500
SI[3]=239200658249xyz+833418885749xz2+833418885749yz2+1103356586250z3-1180278730000xe-1180278730000ye-4122562960000ze-2256930743125x-2256930743125y-3735215937500z
SI[4]=29276712927293877052y3+34502179996697420014y2z-21846789615074696408xz2+12655390381622723606yz2+353923172478567052z3-107050375361942719936xe-93115796510199938704ye-15988357164025778704ze-83875283582948042378x-111376344722279890453y-72625380249515445453z
SI[5]=14638356463646938526xy2-8200223385144770224y2z-176961586239283526xz2-23015541435030992276yz2-19613880879408765000z3+70861567175780760000xe+9958687579002870000ye+62262369924092910000ze+55520908001539886250x+47760192145062486875y+74039012672894254375z
SI[6]=228002467100370827713653799444071601263087585110095658514243152481709891394766940759710105600e4+622420329770799564714444791871544119479819936213130785423343244231693687313045940678952550400e3+506248207039081371311793836716335756860043965099318815883875996821460771462670451574403197xy+506248207039081371311793836716335756860043965099318815883875996821460771462670451574403197xz+506248207039081371311793836716335756860043965099318815883875996821460771462670451574403197yz+582458467577249837175195304160820682747771399906631566857923156855913402521615604464015116800e2+221942917068924121152098427820265166683395127057625211137205725332328446352690831823236240000e+30157659835392355669640529170767126256921238718815782304692198696908552067647797808697526250
SI[7]=13408931136117299633713041709524907507566080460931628689460218652900133529160977133420544ze3+22025521781068565270098490133000324243772455491759667912372905692883781509354990616045xz2+22025521781068565270098490133000324243772455491759667912372905692883781509354990616045yz2-55488028253518376909482595134329041274726669071706114303533581710913564441751728061850z3+3816005222319120513787933291748941720549993871248188376199416142844074610381189994407168xe2+3816005222319120513787933291748941720549993871248188376199416142844074610381189994407168ye2+24041315879060365573281247890004280723751804767965262588550186454686031579774587222823680ze2+4581478820300433380789518644007255136756373226500880394476689926960690040819729950887504xe+4581478820300433380789518644007255136756373226500880394476689926960690040819729950887504ye+14192945230321578314317170617282507973086503369718031306120581152965341874563209385840704ze+1343805444592621060798625328885952183168819941800042233194769293890360792605482346080445x+1343805444592621060798625328885952183168819941800042233194769293890360792605482346080445y+2898189564670601974261961974910970210440038833912590454345264350771475174679960653456070z
SI[8]=1049342723919131517435481505062290686819598758631126466351088331120005749591550587530091511808ye3+7806587755722102896127155036888830744961341564554145687708363777858074062070845150777770650y2z-3219482199841696163289122420022090719504926530290829640576705694756352401884541411106368235xz2+4587105555880406732838032616866740025456415034263316047131658083101721660186303739671402415yz2+2362008026394499694889052921691229844023000009541545713740101914158294382374466289965857950z3+298629120683027414047502295612396932225080870382269477756237709090548746784600785392321746176xe2+1881401256747627028668270616128064996598644985726657554392171941384364773338419872296512725760ye2+298629120683027414047502295612396932225080870382269477756237709090548746784600785392321746176ze2+334311183793041392327338833318808348071189711281052048539023668644589875971870325482043494928xe+1095713740318563505455270362029974190515676856893489001566624294381788211190607609404086934528ye+348830063071248334197307105626001950473691955427752315136272366947789288451060669110875262128ze+86184258329254071865760009626449856132120998254861902390601368471639535206213478820357126815x+204660550962627080698181109945089665832383818789040982898997000681340226362586109491527086190y+85672358169329370488425066381663321445191921294050172717398208295868835334088143377854756815z
SI[9]=1049342723919131517435481505062290686819598758631126466351088331120005749591550587530091511808xe3-7806587755722102896127155036888830744961341564554145687708363777858074062070845150777770650y2z+26198657178752458104320535815514281539587299372747702491774339082026322482958533320105685515xz2+18392069423030355208193380778625450794625957808193556804065975304168248420887688169327914865yz2+34684192359168712778522995554705931336275988393160728530140480085016674806644514293915893750z3+1881401256747627028668270616128064996598644985726657554392171941384364773338419872296512725760xe2+298629120683027414047502295612396932225080870382269477756237709090548746784600785392321746176ye2+298629120683027414047502295612396932225080870382269477756237709090548746784600785392321746176ze2+1052787331261593162442310317662232781883238571043694463317270307957321184512502952628873137328xe+291384774736071049314378788951066939438751425431257510289669682220122849293765668706829697728ye+198893595111621148571650800805184455875348789716162234209295068660078383142713630589720647728ze+122576607712513773380234217484509961780067947212097493169515279755848729788150727450704964965x+4100315079140764547813117165870152079805126677918412661119647546148038631778096779535005590y-42369818586056822777702712018310528883988914380608736268377511784861203931354925307420360035z
SI[10]=5286314127959688365525177032268954392579943701679465656689238382868654088519230830963328000z2e2-1498372741049672898680532532154074834103580369331621493985704807020219033269018747299892000xze-1498372741049672898680532532154074834103580369331621493985704807020219033269018747299892000yze+5049778834731427296286514321733140655002348099348702291880134882436426482803886574326544000z2e-1899635523942244127943296678322265315127878372952214553561963573615378010231894085258240000e3-118481565678500128583946435171007709473615739827672664977906332192758750137955670656549059xy-1122122163146980144160527399392121592426424743581223061706380393521644611290417587716692809xz-1122122163146980144160527399392121592426424743581223061706380393521644611290417587716692809yz+767094159614274743213178752348593807964392065892761224881704692785127061328279770333037500z2-6336794162786484791490850014021867247632536581719166903655938125876307736528689661552640000e2-5652829900328978549906994919430696302123861654447982712706468043799066564611307949954500000e-1500856584379959748684990702625839517372954224443164618608262694397010700820021325594796250
SI[11]=21145256511838753462100708129075817570319774806717862626756953531474616354076923323853312yze2+3521808048377036890306141294225256906828418932505609048560466654639629139925358046420000y2e+27678760162586989418094374773513141475678678584925798272325103346596434372809312821659040yze+3521808048377036890306141294225256906828418932505609048560466654639629139925358046420000z2e+24181699552587089975949496737491470466978157307994456606056132246456753330952400337920000e3+17077143186999212896553545297308162489558750984408807263154505782525542600430982714715xy+2388522432624828867055925739242211404683763497160896378025050052119395665745081761268750y2+17077143186999212896553545297308162489558750984408807263154505782525542600430982714715xz+8676654303676433250170028450782259648651878162557548003053396659540117969320642469818215yz+2388522432624828867055925739242211404683763497160896378025050052119395665745081761268750z2+47550277905468517774720144569254515044542450951525955519065611073100787925576111160960000e2+24879894543203882181887093584586385325051319877070351964838122852660826011218911456300000e+2801601780580562829702207130812724195601705282597427649492207379062660958221322455306250
SI[12]=21145256511838753462100708129075817570319774806717862626756953531474616354076923323853312xze2-3521808048377036890306141294225256906828418932505609048560466654639629139925358046420000y2e+27678760162586989418094374773513141475678678584925798272325103346596434372809312821659040xze+5807408688265243610466040773567680496661361031291496355721605775725580900196654318080000e3+234340226633516503805114942386107230815516399295159411988678798819147201917231700310805xy-2388522432624828867055925739242211404683763497160896378025050052119395665745081761268750y2+8893917387122950541078589847871058716977835810868298607778920952576739628637443187414305xz+234340226633516503805114942386107230815516399295159411988678798819147201917231700310805yz+14607510684846075805524967836709461027054725354294196790222643407324553134319864430720000e2+14666390425623309357574348835682101842396843938016079816756801503007590546868224693050000e+5269905809804186906628687702756015760155118412005009035106702894372127833937730060612500
SI[13]=5286314127959688365525177032268954392579943701679465656689238382868654088519230830963328000y2e2+5049778834731427296286514321733140655002348099348702291880134882436426482803886574326544000y2e+1498372741049672898680532532154074834103580369331621493985704807020219033269018747299892000xze-8914570754734089075685235654321356006346344736672067838968410158520883098357794212618240000e3-22965382607351832345809429831717632729500979924944089393672394352136121317235934601721559xy+767094159614274743213178752348593807964392065892761224881704692785127061328279770333037500y2+980675214861128183230771534389396250223308023828606307334801666976749739835225982458422191xz-22965382607351832345809429831717632729500979924944089393672394352136121317235934601721559yz-18913681079518559504955547616331103523554413265485233609248020540660022942463199510512640000e2-10896696231300768553145829892607650730027798431090334436383526803257286533663637904822000000e-1470397573097166101852680844186913696842716504802932305769562568996792157514170115772921250
SI[14]=32909631983014463271230752612485727999323250727990312064z3e+1726536864896562683771065089147096216066025926565019955xz2+1726536864896562683771065089147096216066025926565019955yz2+27161840744915383963292234851337506401558378338816090130z3-97181425887471889552962684361068076000891868848812124416xe2-97181425887471889552962684361068076000891868848812124416ye2-151827546943190531727111335690292016005077070433074285312ze2-196386641837144315730482926434512597573149198184345973968xe-196386641837144315730482926434512597573149198184345973968ye-308049867339439914014357335666079328455860027543595886848ze-97145914923651157152083576671210258187864628169760407025x-97145914923651157152083576671210258187864628169760407025y-146888449915178393989378838001270812841406515137292092150z
SI[15]=21890977095805484243841992561160012736365836873872871735135808yz2e+1145911992948332694918104845284164225139786664759941496216190y2z+404593650843315133920184031290596144361250001381311948199035xz2+10281330713560539254029090665269009915894972440282201484019925yz2-4152193938699200263184347582186730760597180322120395003802790z3+14316003455913026116999404146995746882037508462474499766106880xe2+50493227316562542417196994175577340756793381616845965532360960ye2+17824469650897128900068250037940003379620622034833926265073920ze2+48295903366877034019167365218535830941808536775664419858304720xe+71430040602160730189162064840140780133725978239576289222398560ye+70323032309652400651214814865075070850619075514632474602454000ze+31718700844898297701187482375345151193814241340731604433674915x+35190733136894653431287924906177727577569775314553717402421540y+45091170316996578152454117660262885498075301207428123980995665z
SI[16]=21890977095805484243841992561160012736365836873872871735135808xz2e-1145911992948332694918104845284164225139786664759941496216190y2z+13453643248280819237784919429846123385145272138774557648830985xz2+3576906185563595117676012795867709613611549699873668113010095yz2+592309014984262717537666974997887145842638625466737403440290z3+50493227316562542417196994175577340756793381616845965532360960xe2+14316003455913026116999404146995746882037508462474499766106880ye2+17824469650897128900068250037940003379620622034833926265073920ze2+65128966625693502137878918692705333999498064841790219038425840xe+41994829390409805967884219071100384807580623377878349674332000ye+48314185142167050798224683644389539032178880483920874009256560ze+23141810106489979640384892497621604350059852228010033682825105x+19669777814493623910284449966789027966304318254187920714078480y+26296138410814499369398816329666371815047695598008637905329355z
SI[17]=21890977095805484243841992561160012736365836873872871735135808y2ze+15401279106014989988878321283917892920991257217097047419490920y2z-3093547850682503446011506699355933760985771743082431266876125xz2+3576906185563595117676012795867709613611549699873668113010095yz2+592309014984262717537666974997887145842638625466737403440290z3+14316003455913026116999404146995746882037508462474499766106880xe2+17824469650897128900068250037940003379620622034833926265073920ye2+50493227316562542417196994175577340756793381616845965532360960ze2+31154832875259704250144722053177609230642973403520787662282000xe+56841556763631245830419017213724178176414457358690876752743920ye+67441591519379408823424082141293470432200137941377778306988480ze+18288461637060596608063467312687192799346985598805975283794105x+27975071056650426957513640648046614457081599862948946683659605y+22844193638087079354491050833343196874983280618451670334779230z
SI[18]=55737986237143195555627467582360237319395758907774300109441454055000z4-196199100724059681407319436100214920715833384026438413892405636956000xze-196199100724059681407319436100214920715833384026438413892405636956000yze-216236142418768723674003071733696546423584719598044122538503443880000z2e+1451748024271672670994554037912340508195838407465353500619437143040000e3+50103323325419523386079919539032099876002034450990127903694667606489xy-192872315751071149147655130483105450374133168028534581766069645679761xz-192872315751071149147655130483105450374133168028534581766069645679761yz-313905160644551271771290095960217752396725699748520112369754403167500z2+2602799617123909601279894361054731251601133408949543411451174845440000e2+1234579763623759527906596903096448346460889613884398457186335989500000e+227046371226329187623544604151156641545969413370867705558994745408750
SI[19]=9289664372857199259271244597060039553232626484629050018240242342500yz3-52232873237732025669855508711518555618365093897293725701214369960000y2e+68600461909673287894329144138957870106290867085732594330680523692000xze-7202045863415706779028664574510886652915187342282867597899564788000yze-19039357121869258764553760848318156901597353493844324714651172500000z2e-345904951611507202027705643439307625819066132381266037924796487680000e3-8012540350013300019850514881496200652564783320392677149373837859913xy-45091365449508976289340323320319966519455146243560447489753704455000y2+48774110674635900776853573998720305096021992762020252339627318363837xz-16207266621586326394583242822994854117851594227336117535433383778663yz-2426142108404410401512976413428979230290493836698658586323831093750z2-620163596273793806942414036004617335680429718727221171633408788480000e2-252117429338412258592117034760643821478708727552834861119290309000000e-5504112774250823567407514763259420034915647620199172583796500448750
SI[20]=27868993118571597777813733791180118659697879453887150054720727027500xz3+156698619713196077009566526134555666855095281691881177103643109880000y2e-21606137590247120337085993723532659958745562026848602793698694364000xze+205801385729019863682987432416873610318872601257197782992041571076000yze+99580548347588300715905243589601196150303221210348202959689592380000z2e-220172848825743707002033694535097049404206227691535045690183265280000e3-1387260902808895066076386038507579167731438804272659572714943356573xy+135274096348526928868020969960959899558365438730681342469261113365000y2-25971439717527974190274569863003539563591871525102980730893581112823xz+168972692171138707324035880602141938078028889442966128894288525314677yz+127995670023313697663482040720672961867493957220585366710289620083750z2-394741922870690649340882527482476950928321694908179400457535022080000e2-301914687874747599296651029270491540957763345221178693783946491500000e-155336221000862978216036360344598766861354767799423539871935543736250
SI[21]=13934496559285798888906866895590059329848939726943575027360363513750y2z2+102582986953112675142083855449520741412570004283195217279701212440000y2e+128498469847991623962971224347320903771267870983601424525030677106000yze+102582986953112675142083855449520741412570004283195217279701212440000z2e+148374037901289755516593411381621004363453371959156495555922951680000e3+5812300779586495311101446371110840409153645944686392498955058039938xy+70725090699491193368652955452855866859252472881481349703398871213750y2+5812300779586495311101446371110840409153645944686392498955058039938xz+102607845154295333151597820831251931816909048961624204568854581700563yz+70725090699491193368652955452855866859252472881481349703398871213750z2+266015784133305084311961850053081471453789074504709518489515092480000e2+55282107177371115160098589589387418588524855830755380692150790250000e-37952656374535168542201850850977216648648741132076097129289388832500

THE GROEBNER BASIS (IN THE LEXICOGRAPHIC MONOMIAL ORDERING) GENERATED BY FGLM ALGORITHM:
j[1]=36812798143709139749144994785898166628646912e5+127499329072859314688739373550168339532546048e4+168144765973871153972385957671411273274218496e3+105507004438312720335072205511167338086667520e2+31442209826685795119941751238920406402581000e+3570217123261998609632303137992216382496875
j[2]=5223155241729446615939982234094518534144z2e4+11826462178341763758803125516807901601792z2e3+9674630135124630527052078934594015491840z2e2+3367827196469529498101185522626133152000z2e+422407904060008292834027766688471040625z2-823425911484652323108207566227537920000e4-1864431545330710644280982077942978560000e3-1525197082722384683921692353164651200000e2-530935047999358288892228768228360000000e-66592241149578807673418427085457031250
j[3]=3683037108272061515125919701641024964091904z3e3+6870355930796712330314622333066809097295872z3e2+4081815576157209090627361527089137653290640z3e+746818480636264240898037984697076691971625z3-4470586803557950016804998343996889169920000ze4-14281273079782202398711256598217495910400000ze3-16038533845100702653365061162476369512320000ze2-7491676367526098069318044436810915291900000ze-1204837027906222365476773974533579201406250z
j[4]=63046886084129596279742524940060664319957725303556417033138206954152670826032321362947238146387500z4-23940852927711156001288974013109566157690065271234421092978078633176194316532217070164127783050878976z2e3-38954662841512101354693962645878061652453771541993478030347914909604810741990018704524306363718931968z2e2-20214162498738635323957961420021615218741600957082639370469790163955477770722677101544570869289670160z2e-3455677668301953521867523331293278593831382997868796316122436690786769587739109991483653802248223375z2+34328112690191248160225811297041940678025435788216774138397787776994980727500111266311554264940544000e4+99234866093704559729585468179288129354277665903411075338757173455332858886455231842925606137854976000e3+98100044732752137387378054721082639959567567933869641031300038754381436242899796913633580898991872000e2+39621942427558920496399735275374974894558657354578296624116445524789909612552160813690925350568500000e+5625000754115883883533486507913189278907557390519665674542936449108326191333311703591615994591718750
j[5]=658740729187721858486566052982030336ye4+1491545236264568515424785662354382848ye3+1220157666177907747137353882531720960ye2+424748038399486631113783014582688000ye+53273792919663046138734741668365625y-658740729187721858486566052982030336ze4-1491545236264568515424785662354382848ze3-1220157666177907747137353882531720960ze2-424748038399486631113783014582688000ze-53273792919663046138734741668365625z
j[6]=7309401854478702737517733525829803316526134925921052880233708522115009878514686132367280yz2e+2915224326296784558140538602006841787691259589716171659178880292051440144323523596655125yz2-51430893181795257258415317445542006409607227458857063896361260629255663672515184660860928ye3-65496010912233703637793760138307234335895694485626318381352534406709669679650646475596544ye2-29593737126207176269929199413546848458282822035060547430241669444160320887355174710429200ye-4647505052685517329520377416223353208301139480669474024744364404875449713634141444124375y-50301950781785441355280212843118240480881892826816456372596519998909457787002205217492480z3e2-52167760089688380621688418448510225199849901815515777407723495645932362108542603228627040z3e-12004672156114132022933368418829393886845403144461514465183528978095267262331787046798500z3-357020705436976405510262189572874805446681549627869043562927457789634118817436888733057024ze4-816306904680338899796105297372324643004195974194723427474153457814597846022225197890879488ze3-613219320874243537352190067962003808530769696177546379552316800803943089471753826823721728ze2-171884714813123191246151955431333394463230510414078258579264557155174215439527329417350400ze-14667545520684401209951574160414186837040467631347953529944303134077139964158082132133125z
j[7]=4849760468009968944595578841543128024612132715658185925626015919550205448156332412534402934337500yz3+708175180799138803667083720242438004070881756916215677120235010756986804842052572438719195722801152yze3+1286909338196414733012587445001605061966184324330454548690744761886901973581941397498214807692481536yze2+755005865096043124025747692178326766449426488812755807842656346560829136060283989248903414183082320yze+135866842123848610828711041199669771897886797697547086107494108189195835436437490393776012519418625yz+1073357517512002067723959611321999190332868920683688721632615574995172528972455737288389046744113152z2e3+1837730737113004100853523649022493404598650363581910594224010817403813944098707878580141244094657536z2e2+999804558665942866009218871318967537667925740826818288985602203799957882777854041223360349474982320z2e+174526677834447667962780889257578150373759285731735878223997394004969087582569873044939093157699875z2-431858837274320756286743884402374793537666182852146458919781655214823468500174370524337398317056000e4-1529068564194684500635014419962987175436376568143181441541929230153482085577784615792444302183424000e3-1728962270281292405152008463735040741022275992597124726668811079644525068702395195623256483294528000e2-764983785071086291169340715120283354431192515776783014237713803150870820971227834888358846771800000e-116157844550031936082422289985550089485958455650618818883325766541794448477240622235794397205625000
j[8]=35517983996072065875302965594726198708653493830230459131210941843923787704126575099359435396215792362500y2+4984218874617104914155008913440529351125858037802285039004339570076607016246742173190041684140057102639104yze3+7905110745868043904633658223114061824382577590842406401226639691617495550493172744003024278762164464986112yze2+4083993177665232544133585141942917292666824157745762593538084425413474821965281665717515862756555703831440yze+723107010629384367421459648808837295330014082701738358522653977685159611505854881968571522852965438779125yz+35517983996072065875302965594726198708653493830230459131210941843923787704126575099359435396215792362500z2-3476255522818816748388604347607992297839198393944678241169969103658937407266647625066096427428111908864000e4-10545537235944524735510339134760949640313018607696167547235936527736740769776817305389644925656922935296000e3-10472948670104601336398053749261186295980902492148297769597285559067800773006233359458362393383253543552000e2-4034269186144752520109288248689978220458989844920818559553895851145995048434712291645836527713190387300000e-564263721947665408786648740126983219046776632962913778443725094131621542673002287662800680761341891406250
j[9]=40105552776408744193070495572680409224060626004488244562247863329844972492170543194635716318131426020701479461552149564375x+40105552776408744193070495572680409224060626004488244562247863329844972492170543194635716318131426020701479461552149564375y+871869994341598760255838471385654770925838702791356066227972547623460589458962875594205364974575738829090311852064153559552z3e2+997313203483818676331608566723764371792644752015642243067972874112720149916296590126351866885226272969164568746634481631840z3e+229124173612030449177094046154959440817662634892948314950195313736232853828259812639718189051704986446085549483592163284125z3+8460527939387913818454105491945483532145918510003735955549929180277303419858823798296949000478233337964018669506468344561664ze4+21918557044773800406073621724288067492013398237322433310919648751979054255638916771060270471776853127184902986799812759773184ze3+18662187776361946431397235513028260621581772014026662066054971720563261099172740600747192731428530621422635945436602584887680ze2+6175305783261312282609977730424118453093763869003569249729415962592576141333406614182025871750063709473919237344997779559000ze+744761297187446660913533931597108832843905489935164322637843490326344462018094558337736006550566649022660126374208472551875z

// 'triang_solve' created a ring, in which a list rlist of numbers (the
// complex solutions) is stored.
// To access the list of complex solutions, type (if the name R was assigned
// to the return value):
        setring R; rlist; 
THE NUMERICAL SOLUTIONS THROUGH TRIANGULATION:
[1]:
   [1]:
-0.39705054600483080889176715350196612593964157002994
   [2]:
-0.39705054600483080889176715350196612593964157002994
   [3]:
-0.39705054600483080889176715350196612593964157002994
   [4]:
-1.1992140197430401395815787932887349116713900566735
[2]:
   [1]:
0.39705054600483080889176715350196612593964157002994
   [2]:
0.39705054600483080889176715350196612593964157002994
   [3]:
0.39705054600483080889176715350196612593964157002994
   [4]:
-1.1992140197430401395815787932887349116713900566735
[3]:
   [1]:
0
   [2]:
1.0626278551055638166791772679717934898300074617838
   [3]:
-1.0626278551055638166791772679717934898300074617838
   [4]:
-0.39883213214095405031135526651863929057839208322827
[4]:
   [1]:
1.0626278551055638166791772679717934898300074617838
   [2]:
0
   [3]:
-1.0626278551055638166791772679717934898300074617838
   [4]:
-0.39883213214095405031135526651863929057839208322827
[5]:
   [1]:
0
   [2]:
-1.0626278551055638166791772679717934898300074617838
   [3]:
1.0626278551055638166791772679717934898300074617838
   [4]:
-0.39883213214095405031135526651863929057839208322827
[6]:
   [1]:
-1.0626278551055638166791772679717934898300074617838
   [2]:
0
   [3]:
1.0626278551055638166791772679717934898300074617838
   [4]:
-0.39883213214095405031135526651863929057839208322827
[7]:
   [1]:
1.0626278551055638166791772679717934898300074617838
   [2]:
-1.0626278551055638166791772679717934898300074617838
   [3]:
0
   [4]:
-0.39883213214095405031135526651863929057839208322827
[8]:
   [1]:
-1.0626278551055638166791772679717934898300074617838
   [2]:
1.0626278551055638166791772679717934898300074617838
   [3]:
0
   [4]:
-0.39883213214095405031135526651863929057839208322827
[9]:
   [1]:
0.54633354693865514425805809740503653829644001345727
   [2]:
0.54633354693865514425805809740503653829644001345727
   [3]:
-1.2729815146351792875086125608150899381682291666662
   [4]:
-0.35306595070499197298391211554480257979649053447805
[10]:
   [1]:
1.2729815146351792875086125608150899381682291666662
   [2]:
-0.54633354693865514425805809740503653829644001345727
   [3]:
-0.54633354693865514425805809740503653829644001345727
   [4]:
-0.35306595070499197298391211554480257979649053447805
[11]:
   [1]:
-0.54633354693865514425805809740503653829644001345727
   [2]:
1.2729815146351792875086125608150899381682291666662
   [3]:
-0.54633354693865514425805809740503653829644001345727
   [4]:
-0.35306595070499197298391211554480257979649053447805
[12]:
   [1]:
0.54633354693865514425805809740503653829644001345727
   [2]:
-1.2729815146351792875086125608150899381682291666662
   [3]:
0.54633354693865514425805809740503653829644001345727
   [4]:
-0.35306595070499197298391211554480257979649053447805
[13]:
   [1]:
-1.2729815146351792875086125608150899381682291666662
   [2]:
0.54633354693865514425805809740503653829644001345727
   [3]:
0.54633354693865514425805809740503653829644001345727
   [4]:
-0.35306595070499197298391211554480257979649053447805
[14]:
   [1]:
-0.54633354693865514425805809740503653829644001345727
   [2]:
-0.54633354693865514425805809740503653829644001345727
   [3]:
1.2729815146351792875086125608150899381682291666662
   [4]:
-0.35306595070499197298391211554480257979649053447805
[15]:
   [1]:
(0.9794595518740171742238918106017120355133512559226+I*0.11513384761218296745950531095862180293656933894103)
   [2]:
(0.9794595518740171742238918106017120355133512559226+I*0.11513384761218296745950531095862180293656933894103)
   [3]:
(-1.3239108228942634760950168298645904839341275797953+I*0.78030189852255354574721590569852587875226700375377)
   [4]:
(-0.75616953738705355659118056081760892651941323671625-I*0.050264825202602481083685002985152452622399276285575)
[16]:
   [1]:
(1.3239108228942634760950168298645904839341275797953-I*0.78030189852255354574721590569852587875226700375377)
   [2]:
(-0.9794595518740171742238918106017120355133512559226-I*0.11513384761218296745950531095862180293656933894103)
   [3]:
(-0.9794595518740171742238918106017120355133512559226-I*0.11513384761218296745950531095862180293656933894103)
   [4]:
(-0.75616953738705355659118056081760892651941323671625-I*0.050264825202602481083685002985152452622399276285575)
[17]:
   [1]:
(-0.9794595518740171742238918106017120355133512559226-I*0.11513384761218296745950531095862180293656933894103)
   [2]:
(1.3239108228942634760950168298645904839341275797953-I*0.78030189852255354574721590569852587875226700375377)
   [3]:
(-0.9794595518740171742238918106017120355133512559226-I*0.11513384761218296745950531095862180293656933894103)
   [4]:
(-0.75616953738705355659118056081760892651941323671625-I*0.050264825202602481083685002985152452622399276285575)
[18]:
   [1]:
(0.9794595518740171742238918106017120355133512559226+I*0.11513384761218296745950531095862180293656933894103)
   [2]:
(-1.3239108228942634760950168298645904839341275797953+I*0.78030189852255354574721590569852587875226700375377)
   [3]:
(0.9794595518740171742238918106017120355133512559226+I*0.11513384761218296745950531095862180293656933894103)
   [4]:
(-0.75616953738705355659118056081760892651941323671625-I*0.050264825202602481083685002985152452622399276285575)
[19]:
   [1]:
(-1.3239108228942634760950168298645904839341275797953+I*0.78030189852255354574721590569852587875226700375377)
   [2]:
(0.9794595518740171742238918106017120355133512559226+I*0.11513384761218296745950531095862180293656933894103)
   [3]:
(0.9794595518740171742238918106017120355133512559226+I*0.11513384761218296745950531095862180293656933894103)
   [4]:
(-0.75616953738705355659118056081760892651941323671625-I*0.050264825202602481083685002985152452622399276285575)
[20]:
   [1]:
(-0.9794595518740171742238918106017120355133512559226-I*0.11513384761218296745950531095862180293656933894103)
   [2]:
(-0.9794595518740171742238918106017120355133512559226-I*0.11513384761218296745950531095862180293656933894103)
   [3]:
(1.3239108228942634760950168298645904839341275797953-I*0.78030189852255354574721590569852587875226700375377)
   [4]:
(-0.75616953738705355659118056081760892651941323671625-I*0.050264825202602481083685002985152452622399276285575)
[21]:
   [1]:
(0.9794595518740171742238918106017120355133512559226-I*0.11513384761218296745950531095862180293656933894103)
   [2]:
(0.9794595518740171742238918106017120355133512559226-I*0.11513384761218296745950531095862180293656933894103)
   [3]:
(-1.3239108228942634760950168298645904839341275797953-I*0.78030189852255354574721590569852587875226700375377)
   [4]:
(-0.75616953738705355659118056081760892651941323671625+I*0.050264825202602481083685002985152452622399276285575)
[22]:
   [1]:
(1.3239108228942634760950168298645904839341275797953+I*0.78030189852255354574721590569852587875226700375377)
   [2]:
(-0.9794595518740171742238918106017120355133512559226+I*0.11513384761218296745950531095862180293656933894103)
   [3]:
(-0.9794595518740171742238918106017120355133512559226+I*0.11513384761218296745950531095862180293656933894103)
   [4]:
(-0.75616953738705355659118056081760892651941323671625+I*0.050264825202602481083685002985152452622399276285575)
[23]:
   [1]:
(-0.9794595518740171742238918106017120355133512559226+I*0.11513384761218296745950531095862180293656933894103)
   [2]:
(1.3239108228942634760950168298645904839341275797953+I*0.78030189852255354574721590569852587875226700375377)
   [3]:
(-0.9794595518740171742238918106017120355133512559226+I*0.11513384761218296745950531095862180293656933894103)
   [4]:
(-0.75616953738705355659118056081760892651941323671625+I*0.050264825202602481083685002985152452622399276285575)
[24]:
   [1]:
(0.9794595518740171742238918106017120355133512559226-I*0.11513384761218296745950531095862180293656933894103)
   [2]:
(-1.3239108228942634760950168298645904839341275797953-I*0.78030189852255354574721590569852587875226700375377)
   [3]:
(0.9794595518740171742238918106017120355133512559226-I*0.11513384761218296745950531095862180293656933894103)
   [4]:
(-0.75616953738705355659118056081760892651941323671625+I*0.050264825202602481083685002985152452622399276285575)
[25]:
   [1]:
(-1.3239108228942634760950168298645904839341275797953-I*0.78030189852255354574721590569852587875226700375377)
   [2]:
(0.9794595518740171742238918106017120355133512559226-I*0.11513384761218296745950531095862180293656933894103)
   [3]:
(0.9794595518740171742238918106017120355133512559226-I*0.11513384761218296745950531095862180293656933894103)
   [4]:
(-0.75616953738705355659118056081760892651941323671625+I*0.050264825202602481083685002985152452622399276285575)
[26]:
   [1]:
(-0.9794595518740171742238918106017120355133512559226+I*0.11513384761218296745950531095862180293656933894103)
   [2]:
(-0.9794595518740171742238918106017120355133512559226+I*0.11513384761218296745950531095862180293656933894103)
   [3]:
(1.3239108228942634760950168298645904839341275797953+I*0.78030189852255354574721590569852587875226700375377)
   [4]:
(-0.75616953738705355659118056081760892651941323671625+I*0.050264825202602481083685002985152452622399276285575)
// ** loaded /usr/bin/../share/singular/LIB/triang.lib (4.1.1.0,Dec_2017)
THE PRIMARY IDEAL DECOMPOSITION THROUGH TRIANGULATION (IN THE LEXICOGRAPHIC MONOMIAL ORDERING):
[1]:
   _[1]=19607184e+7819975
   _[2]=1107z3-1250z
   _[3]=1107y2+1107yz+1107z2-1250
   _[4]=x+y+z
[2]:
   _[1]=33596906582185481529961979904e3+62671838378960619969574479872e2+37234589977346832313644870640e+6812527267627204196782565375
   _[2]=87306551258263729827909084908235z2-614312087531946676701270123361536e2-537304333596464593384375038355328e-139185734162956356442927812890825
   _[3]=331997850486797035543167841067099398038750y2-13015916170638763880890008092932038290847744yze2-13459096677815806942752983709330245786664480yze-2687870434415068556840506490446894349472000yz+11262181386982462508243034408486017150784000e2+12991002284039358505441186364021967659282000e+2951891604844851948796638575554228299190625
   _[4]=18444325027044279752398213392616633224375x+18444325027044279752398213392616633224375y-723106453924375771160556005162891016158208ze2-747727593211989274597387983851680321481360ze-149326135245281586491139249469271908304000z
[3]:
   _[1]=55883592e+67016387
   _[2]=7929z2-1250
   _[3]=y-z
   _[4]=x-z
[4]:
   _[1]=33596906582185481529961979904e3+62671838378960619969574479872e2+37234589977346832313644870640e+6812527267627204196782565375
   _[2]=87306551258263729827909084908235z2+8514144339559070475415581022605696e2+9287598840997447194191617733989768e+2076320747503839544988065579439950
   _[3]=54922323119969587357485501941034906122670y+1008818016691184154099544389734581696829952ze2+1101539894576580693998431276321064052056416ze+286732811316955459193115321222624363426985z
   _[4]=54922323119969587357485501941034906122670x+1008818016691184154099544389734581696829952ze2+1101539894576580693998431276321064052056416ze+286732811316955459193115321222624363426985z
Auf Wiedersehen.
\end{Verbatim}
